# Supplementary material for: Tight convergence rates of the gradient method on smooth hypoconvex functions
Source: arXiv:2203.00775 source file (2022-06-21)
Supplement: Supplementary file 1 [file A8_Numerical_Experiments.tex]

%!TEX root = ../../main.tex
\clearpage
\subsection{Setup of numerical experiments}\label{appendix:experiments}

\subsubsection{$l_0$-regularization}

\paragraph{Lasry-Lions envelope.} To smooth a nonsmooth and nonconvex function, one can use the Lasry-Lions double envelope \cite{Lasry1986}, \cite[Example 1.46]{RockafellarW98_Var_Analysis}. Given a $\gamma_f$-proximal bounded function $f$, i.e., $f+\tfrac{1}{2\gamma} \|\cdot\|^2$ is bounded for all $\gamma < \gamma_f$, and $0 < \sigma < \lambda < \gamma_f$, the Lasry-Lions double envelope is defined as 
$e_{\lambda,\sigma} f(x):=\sup \limits _w \inf \limits _u \big\{  f(u) + \tfrac{1}{2\lambda}\|u-w\|^2 - \tfrac{1}{2\sigma}\|w-x\|^2  \big\}$ and is smooth. 

In the particular case of $l_0$ regularization, the analytical computations are given in \cite[Example II.5]{Simoes_on_Lasry_Lions_Env_2021}.
With some abuse of notation, let the $l_0$ regularization function $l_0:\mathbb{R} \rightarrow \mathbb{R}$, 
\begin{align*}
    l_0(x)=|x|_0 = \left\{
    \begin{array}{ll}
        1 & x \neq 0 \\
        0 & x = 0
    \end{array}
    \right.. 
\end{align*}
Then
\begin{align*}
\begin{aligned}
    e_{\lambda,\sigma} l_0(x) &= \left\{
    
    \begin{array}{ll}
        \tfrac{1}{2(\lambda-\sigma)} x^2 
            & |x| \leq \big(1-\tfrac{\sigma}{\lambda}\big) \sqrt{2 \lambda} \\
        1 - \tfrac{1}{2 \sigma} \big(|x| - \sqrt{2\lambda}\big)^2 
            & |x| \in \big[ \big(1-\tfrac{\sigma}{\lambda}\big) \sqrt{2 \lambda}\,,\, \sqrt{2 \lambda} \big] \\
        1 
            & |x| \geq \sqrt{2 \lambda}
    \end{array}
    \right. \\
    \nabla e_{\lambda,\sigma} l_0(x) &= \left\{
    
    \begin{array}{ll}
        \tfrac{1}{\lambda-\sigma} x
            & |x| \leq \big(1-\tfrac{\sigma}{\lambda}\big) \sqrt{2 \lambda} \\
        -\tfrac{1}{\sigma} \big(|x| - \sqrt{2\lambda}\big)
            & |x| \in \big[ \big(1-\tfrac{\sigma}{\lambda}\big) \sqrt{2 \lambda}\,,\, \sqrt{2 \lambda} \big] \\
        0
            & |x| \geq \sqrt{2 \lambda}
    \end{array}
    \right.
\end{aligned}
\end{align*}
One can notice that $e_{\lambda,\sigma} \in \mathcal{F}_{-\sigma^{-1}, (\lambda-\sigma)^{-1}}$.

%%%%%%%%%%%%%%%%%%%%%%%%%%%%%%%%%%%%%%%%%%%%%%%%%%%%%%%%%%%%%%%%%%%%%%%%%%%%%%%%
\subsubsection{One-dimensional Huber loss}
Assume we have a data matrix $A \in \mathbb{R}^{N \times d}$, where $d$ is the number of features, and $y \in \mathbb{R}^N$ is the associated vector of, for example, labels. By $A_i$ are denoted the rows of $A$ and $x \in \mathbb{R}^d$ is the optimization variable.

\paragraph{Huber loss.}
One-dimensional Huber function, with $\delta > 0$:
\begin{align*}
    H_{\delta}(w) &= \left\{
    
    \begin{array}{cc}
        \frac{1}{2\delta} w^2 \,, & \text{ if } |w| \leq \delta \\
         |w| - \frac{\delta}{2} \,, & \text{ if } |w| > \delta
    \end{array}
    \right. \\
    \nabla_w H_{\delta}(w) &= \left\{
    
    \begin{array}{cc}
        \frac{1}{\delta} w \,, & \text{ if } |w| \leq \delta \\
         \sgn(w) \,, & \text{ if } |w| > \delta
    \end{array}
    \right. \\
    H_{\delta}(w) &\in \mathcal{F}_{0, {\delta}^{-1}}
\end{align*}
When $w = \|Ax - b\|_2$,
\begin{align*}
    H_{\delta}(\|Ax - b\|_2) &= \left\{
    
    \begin{array}{cc}
        \frac{1}{2\delta} \|Ax-b\|_2^2 \,, & \text{ if } \|Ax-b\|_2 \leq \delta \\
         \|Ax-b\|_2 - \frac{\delta}{2} \,, & \text{ if } \|Ax-b\|_2 > \delta
    \end{array}
    \right. \\
    \nabla_x H_{\delta}(\|Ax - b\|_2) &= \left\{
    
    \begin{array}{cc}
        \frac{1}{\delta} A^T (Ax-b) \,, & \text{ if } \|Ax-b\|_2 \leq \delta \\
         A^T \frac{Ax-b}{\|Ax-b\|_2} \,, & \text{ if } \|Ax-b\|_2 > \delta
    \end{array}
    \right. \\
    H_{\delta}(\|Ax-b\|_2) &\in \mathcal{F}_{0, \delta^{-1}\, \|A^T A\|_2}
\end{align*}

\paragraph{Adding $l_2$-regularization.} By adding a curvature $\mu$, we obtain the function
\begin{align*}
    f(x) &= H_{\delta} (\|Ax-b\|_2) + \frac{1}{2} \mu \|x\|^2 \\
    \nabla f(x) &= \nabla H_{\delta} (\|Ax-b\|_2) + \mu x \\
    f & \in \mathcal{F}_{\mu,\, \delta^{-1}\, \|A^T A\|_2 + \mu}
\end{align*}
with
\begin{align*}
    \kappa = \frac{\mu}{\delta^{-1}\, \|A^T A\|_2 + \mu}  \Leftrightarrow
    \frac{1}{\kappa} = \frac{1}{\mu^{-1} \, \delta^{-1}\, \|A^T A\|_2 + 1}.
\end{align*}
For a fixed $\kappa$ we get the curvatures:
\begin{align*}
    \mu &= \frac{\kappa}{1-\kappa} \delta^{-1}\, \|A^T A\|_2 \\
    L   &= \frac{1}{1-\kappa}  \delta^{-1}\, \|A^T A\|_2.
\end{align*}

\begin{figure}[H]
    \centering
    \includegraphics[width=\textwidth]{pics_misc/Huber_convex.eps}
    \caption{The convex case: the larger the better - follows Proposition 4.3 based on the Conjecture for the third regime!}
\end{figure}

\begin{figure}[H]
    \centering
    \includegraphics[width=\textwidth]{pics_misc/Huber_kappa=-0.5.eps}
    \caption{With $\kappa=-0.5$ -- strange convergence...}
\end{figure}

% Alternatively (not equivalent?!),
% \begin{align*}
%     H_{\delta}(Ax-b) &= \left\{
%     \def\arraystretch{1.5}
%     \begin{array}{cc}
%         \frac{1}{2} \|Ax-b\|^2 \,, & \text{ if } \|Ax-b\| \leq \delta \\
%          \delta\, (\|Ax-b\| - \frac{\delta}{2}) \,, & \text{ if } \|Ax-b\| > \delta
%     \end{array}
%     \right. \\
%     \nabla_x H_{\delta}(Ax-b) &= \left\{
%     \def\arraystretch{1.5}
%     \begin{array}{cc}
%         A^T (Ax-b) \,, & \text{ if } \|Ax-b\| \leq \delta \\
%          \delta\, A^T \frac{Ax-b}{\|Ax-b\|} \,, & \text{ if } \|Ax-b\| > \delta
%     \end{array}
%     \right. \\
%     H_{\delta}(Ax-b) &\in \mathcal{F}_{0, \|A^T A\|}
% \end{align*}

% Element-wise Huber function, which is just element-wise smooth (!):
% \begin{align*}
%     H_{\delta}([Ax-b]_i) &= \left\{
%     \def\arraystretch{1.5}
%     \begin{array}{cc}
%         \frac{1}{\delta} ([Ax-b]_i)^2 \,, & \text{ if } |[Ax-b]_i| \leq \delta \\
%          \delta (|[Ax-b]_i| - \frac{\delta}{2}) & \text{ if } |[Ax-b]_i| > \delta
%     \end{array}
%     \right. \\
%     \nabla_x H_{\delta}(Ax-b) &= \left\{
%     \def\arraystretch{1.5}
%     \begin{array}{cc}
%         A_i^T [Ax-b]_i \,, & \text{ if } \|Ax-b\| \leq \delta \\
%         \delta \sgn ([Ax-b]_i) \,, & \text{ if } \|Ax-b\| > \delta
%     \end{array}
%     \right. \\
%     H = \sum_{i=1}^{N} H_{\delta}(Ax-b)
% \end{align*}

%%%%%%%%%%%%%%%%%%%%%%%%%%%%%%%%%%%%%%%%%%%%%%%%%%%%%%%%%%%%%%%%%%%%%%%%%%%%%%%%
\clearpage
\subsubsection*{Binary logistic regression with $l_0$-regularization}
\paragraph{Binary logistic regression. } Using the sigmoid function $\sigma(x) := \big(1+exp(-x)\big)^{-1}$, the loss reads
\begin{align*}
    \begin{aligned}
        \mathcal{L}(x) = -\tfrac{1}{N} \sum_{i=1}^N y_i \log \big(\sigma(A_i x)\big) + (1-y_i) \log \big(1-\sigma(A_i x)\big).
    \end{aligned}
\end{align*}
Its gradient and hessian are given by
\begin{align*}
    \begin{aligned}
        \nabla_x \mathcal{L}(x) &= \tfrac{1}{N} A^T \big(\sigma(A_i x) - y\big) \\
        \nabla^2_x \mathcal{L}(x) &= \tfrac{1}{N} A^T B A
    \end{aligned}
\end{align*}
where $B$ is a diagonal matrix with $B_{i,i}=\sigma(A_i x)(1-\sigma(A_i x))$. 
The loss function $\mathcal{L}$ is convex (not strongly-convex) and its Lipschitz constant is approximated by its upper bound:
\begin{align*}
    L_{\mathcal{L}} = \|\tfrac{1}{N} A^T B A\| \leq \tfrac{1}{N} \|A^T A\|.
\end{align*}

\paragraph{Adding $l_0$ regularization. } The $l_0$ regularization is used to enforce sparsity in the solution. However, because $l_0$ is nonsmooth, it has to be approximated. One approach is involving the Lasry-Lions double envelope $e_{\lambda,\sigma} l_0(x)$. Then we want to
\begin{align*}
    \begin{aligned}
        \minimize_x f(x) := \mathcal{L}(x) + l_0(x) \approx \mathcal{L}(x) + \beta e_{\lambda,\sigma} l_0(x)
    \end{aligned}
\end{align*}
where $\beta$ is a regularization parameters. The function $f$ and its gradient are given explicitly as
\begin{align*}
    \begin{aligned}
        f(x) &= 
        -\tfrac{1}{N} \sum_{i=1}^N y_i \log \big(\sigma(A_i x)\big) + (1-y_i) \log \big(1-\sigma(A_i x)\big) +
        \beta \sum_{i=1}^N e_{\lambda,\sigma} l_0([x]_i) \\
        \nabla f(x) &= 
        \tfrac{1}{N} A^T \big(\sigma(A_i x) - y\big) + \beta \nabla e_{\lambda,\sigma} l_0(x)
    \end{aligned}
\end{align*}
Denoting the lower and upper curvatures of $f$ by $\mu$ and $L$, i.e., $f \in \mathcal{F}_{\mu,L}$, they are:
\begin{align*}
    \begin{aligned}
        \relax [\mu,L] = [0, L_{\mathcal{L}}] + \beta[-\tfrac{1}{\sigma}, \tfrac{1}{\lambda - \sigma}] 
                % \\ &= [-\tfrac{\beta}{\sigma}, L_{\mathcal{L}} + \tfrac{\beta}{\lambda - \sigma}] \\
                \approx [-\tfrac{\beta}{\sigma}, \tfrac{1}{N} \|A^T A\| + \tfrac{\beta}{\lambda - \sigma}] 
    \end{aligned}
\end{align*}

%%%%%%%%%%%%%%%%%%%%%%%%%%%%%%%%%%%%%%%%%%%%%%%%%%%%%%%%%%%%%%%%%%%%%%%%%%%%%%%%
