# Supplementary material for: Tight convergence rates of the gradient method on smooth hypoconvex functions
Source: arXiv:2203.00775 source file (2022-06-21)
Supplement: Supplementary file 2 [file Appendix_Rate.tex]

%%%%%%%%%%%%%%%%%%%%%%%%%%%%%%%%%%%%%%%%%%%%%%%%%%%%%%%%%%%%%%%%%%%%%%%%%%%%%%%
% \clearpage
This section proves the central result of the paper, the convergence rate for smooth hypoconvex functions, i.e., Theorem \ref{thm:wc_GM_hypo}.
\begin{proof}
We consider a feasible point $(l,x_0,\{(g_i,f_i)\}_{i \in \mathcal{I}})$ of problem \eqref{eq:PEP_quad}
{\small
\begin{align*}
    \begin{aligned}
        \maximize_{l\,,\,x_0\,,\,\{(g_i,f_i)\}_{i \in \mathcal{I}}} \quad & l \\
        \stt \quad &
        f_{i}-f_{j}-\langle g_{j}, x_{i}-x_{j}\rangle 
    {}\geq{} 
        \tfrac{1}{2(1-\kappa)}\big(\tfrac{1}{L}\|g_{i}-g_{j}\|^{2} + \kappa L\|x_{i}-x_{j}\|^2-
        2 \kappa \langle g_{j}-g_{i}, x_{j}-x_{i}\rangle\big) \,\, \forall i,j \in \mathcal{I} \\
        \quad & x_{i+1}=x_{i}-\tfrac{1}{L} h_i g_{i}, \quad i \in\{0, \ldots, N-1\} \\
        \quad & f_i- \tfrac{1}{2L}\|g_i\|^2 - f_* {}\geq{} 0, \quad i \in\{0, \ldots, N\} \\
        \quad & f_*-f_{0}-\Delta {}\geq{} 0 \\
        \quad & \|g_{i}\|^2 - l {}\geq{} 0, \quad 0 {}\leq{} i {}\leq{} N
    \end{aligned}
\end{align*}
}%
and show that the right-hand-side of \eqref{eq:GM_hypo_rate_both},
{\normalsize
\begin{align*}
    U =
        \frac{2L\Delta}{1 + 
        \sum\limits_{i=0}^{N-1} \left[2 h_i -
        h_i^2 \frac{-\kappa}{
        2 \min\left(1, \frac{1}{h_i}\right) - (1+\kappa)} 
        \right]}
\end{align*}
}%
is an upper bound of $l$.

The dual values were identified using the PESTO toolbox \cite{PESTO} and only the active constraints were selected for the proof, i.e., the ones with non-zero multipliers. The following inequalities are active:
\begin{enumerate}
    \item \textbf{Interpolability conditions} -- only for adjacent pairs $(i,i+1)$ and $(i+1,i)$
    \begin{enumerate}
        \item $(i,i+1)$ with the \textbf{dual multipliers $\alpha_i$}
        {\normalsize
        \begin{align*}
        \hspace{-0.2in}
        f_{i}-f_{i+1} + \tfrac{-h_i}{(1-\kappa)L} \langle g_{i}, g_{i+1}\rangle 
        -\tfrac{1}{2(1-\kappa)L} \|g_{i}-g_{i+1}\|^{2} +
        \tfrac{\kappa h_i (2 - h_i)}{2(1-\kappa)L} \|g_i\|^2    {}\geq{} 0
    \end{align*}
    }%
        \item $(i+1,i)$ with the \textbf{dual multipliers $\alpha_i-B$}; not active for $h_i \in (0,1]$
        {\normalsize
        \begin{align*}
        \hspace{-0.2in}
     f_{i+1} - f_i
        + \tfrac{-h_i \kappa}{(1-\kappa)L} \langle g_{i}, g_{i+1} \rangle
        - \tfrac{1}{2(1-\kappa)L} \|g_{i}-g_{i+1}\|^2
        + \tfrac{h_i(2-\kappa h_i)}{2(1-\kappa)L} \|g_i\|^2
        {}\geq{} 0
    \end{align*}
    }%
    \end{enumerate}
    \item \textbf{Optimality conditions} -- only for $i=N$, with the \textbf{dual multiplier $B$}
    {\normalsize
    \begin{align*}
         f_N - f_* - \tfrac{1}{2L}\|g_N\|^2 {}\geq{} 0
    \end{align*}
    }%
    \item \textbf{Initial condition} -- with the \textbf{dual multiplier $B$}
    {\normalsize
    \begin{align*}
         f_* - f_0 + \Delta {}\geq{} 0
    \end{align*}
    }%
    \item \textbf{Performance measure} -- with \textbf{dual multipliers $\sigma_i$}
    {\normalsize
    \begin{align*}
        \|g_{i}\|^2 - l {}\geq{} 0, \quad 0 {}\leq{} i {}\leq{} N
    \end{align*}
    }%
\end{enumerate}
We found $B := \tfrac{U}{\Delta}$. For $h_i \in \big(0, 1\big]$, the dual multipliers are:
{\normalsize
\begin{align}
    & \alpha_i = B\,\,,   \quad i = 0,\dots,N-1 \\
    & \sigma_0 
    = \tfrac{h_0 B}{L} \left[1 - \tfrac{1 - \kappa h_0}{2(1-\kappa)}\right] \label{eq:sigma_0_gL_leq_1} \\
    & \sigma_i 
    = \tfrac{h_i B}{L} \left[1 - \tfrac{1 - \kappa h_i}{2(1-\kappa)}\right] + 
    \tfrac{h_{i-1} B}{L} \tfrac{1}{2(1-\kappa)}\,\,,  \quad i = 1,\dots,N-1 \label{eq:sigma_i_gL_leq_1} \\
    & \sigma_N = 1 - \sum\limits_{i=0}^{N-1} \sigma_i = \tfrac{B}{2L} + \tfrac{h_{N-1} B}{L} \tfrac{1}{2(1-\kappa)}\label{eq:sigma_N_gL_leq_1}
\end{align}
}%
For $h_i \in \big[1, \bar{h}(\kappa)\big]$, the \textit{non-negative} dual multipliers are:
{\normalsize
\begin{align}
    & \alpha_i = B\ \tfrac{1-\kappa h_i}{2-(1+\kappa)h_i}\,\, , \quad i = 0,\dots,N-1 \label{eq:alpha_i_gL_geq_1}\\
    & \sigma_0 
    = \tfrac{h_0 B}{L} \left[1 - \tfrac{1-\kappa h_0^2}{2\left[2-(1+\kappa)h_0\right]} \right] \label{eq:sigma_0_gL_geq_1}\\ 
    & \sigma_i 
    = \tfrac{h_i B}{L} \left[1 - \tfrac{1-\kappa h_i^2}{2\left[2-(1+\kappa)h_i\right]} \right] + \tfrac{h_{i-1} B}{L} \tfrac{1}{2\left[2-(1+\kappa)h_{i-1}\right]}\,\, , \quad i=1,\dots,N-1 \label{eq:sigma_i_gL_geq_1}\\
    & \sigma_N 
    = 1 - \sum\limits_{i=0}^{N-1} \sigma_i  
    = \tfrac{B}{2L} + \tfrac{h_{N-1} B}{L}\tfrac{1}{2\big[2-(1+\kappa)h_{N-1}\big]}
\end{align}
}%
The non-negativity of the multipliers leads to the \textbf{threshold} $\bar{h}(\kappa)$. Because $h_i>0$, $2-(1+\kappa)h_i>0$ (from $\kappa {}\leq{} 0$ and $h_i < 2$) and $B>0$, these three non-negativity conditions for $h_i \in \big[1, \bar{h}(\kappa)\big]$ can be rewritten as:
{\normalsize
\begin{align*}
\begin{aligned}
    \big[2-(1+\kappa)h_i\big]\tfrac{2L \alpha_i}{h_i B} 
    {}&={} 1-\kappa h_i {}\geq{} 0 \\
    \big[2-(1+\kappa)h_0\big]\tfrac{2L \sigma_0}{h_0 B}
    {}&={} \kappa h_0^2 - 2(1+\kappa)h_0 + 3
    {}\geq{} 0 \\
    \big[2-(1+\kappa)h_i\big]\tfrac{2L \sigma_i}{h_i B}
    {}&={}  \kappa h_i^2 - 2(1+\kappa)h_i + 3 + \tfrac{h_{i-1}}{h_i} \tfrac{2-(1+\kappa)h_i}{2-(1+\kappa)h_{i-1}}
    {}\geq{} 0
\end{aligned}    
\end{align*}
}%
The first inequality is valid because $\kappa < 0$. The fraction from the last inequality is positive, but can be arbitrarily small because of $h_{i-1}$ and hence the worst-case to analyze is the same as for $\sigma_0$. Therefore, a sufficient condition is
{\normalsize
\begin{align*}
\begin{aligned}
    \kappa h_i^2 - 2(1+\kappa)h_i + 3 {}\geq{} 0, \\
\end{aligned}
\end{align*}
}%
leading to the condition $h {}\leq{} \bar{h}(\kappa)= \tfrac{1+\kappa-\sqrt{1-\kappa+\kappa^2}}{\kappa}$.

Following the idea of \cite[Theorem 2]{abbaszadehpeivasti2021GM_smooth}, showing $l {}\leq{} U$ is equivalent with proving that adding non-negative terms to $l-U$ keeps the difference non-positive. More specifically,
{\normalsize
\begin{align*}%\label{eq:dual_upper_bound}
\begin{aligned}
    l-U 
    & +\sum\limits_{i=0}^N \sigma_i\ \big(\|g_{i}\|^2 - l\big) \\ 
    & +B\ \big(f_* - f_0 + \Delta\big) + \\
    & +B\ \big(f_N - f_* - \tfrac{1}{2L}\|g_N\|^2 \big) + \\
    & +\sum\limits_{i=0}^{N-1} \alpha_i\ 
    \big[ f_{i}-f_{i+1} + \tfrac{-h_i}{(1-\kappa)L} \langle g_{i}, g_{i+1}\rangle 
        -\tfrac{1}{2(1-\kappa)L} \|g_{i}-g_{i+1}\|^{2} +
        \tfrac{\kappa h_i (2 - h_i)}{2(1-\kappa)L}
        \|g_i\|^2
        \big]  + \\
    & + \sum\limits_{i=0}^{N-1} \big(\alpha_i-B\big)\ 
    \big[ 
     f_{i+1} - f_i
        + \tfrac{-h_i \kappa}{(1-\kappa)L} \langle g_{i}, g_{i+1} \rangle
        - \tfrac{1}{2(1-\kappa)L} \|g_{i}-g_{i+1}\|^2
        + \tfrac{h_i(2-\kappa h_i)}{2(1-\kappa)L} \|g_i\|^2
     \big]         
        {{}\leq{}} 0
\end{aligned}
\end{align*}
}%
The proof is based on basic algebraic manipulations. The main idea is to form squares in the left hand side of the inequality. First, we apply some straightforward simplifications, extract the term corresponding to $i=N$ and group the terms with respect to the gradients.
{\normalsize
\begin{align*}
\begin{aligned}
    % & \tfrac{h_0}{L}
    % \left\{
    % \Big[
    % -(1+\kappa)\alpha_0+\kappa B
    % \Big]  \langle g_{0}, g_{1}\rangle -
    % \tfrac{2\alpha_0 - B}{2h_0} \|g_{0}-g_{1}\|^{2}
    % +
    % % \right. \\ & \left. \qquad  \qquad
    % \Big[\tfrac{- (2\alpha_0 - B) \kappa h_0 }{2} + (1+\kappa)\alpha_0-B + 
    % \tfrac{(1-\kappa)L}{h_0}\sigma_0
    % \Big] \|g_0\|^2
    % \right\} + \\
    %%%%
    %%%%
    \sum\limits_{i=0}^{N-1} & \tfrac{h_i}{L} \left\{
    \Big[-\left(1+\kappa\right)\alpha_i+\kappa B \Big] \langle g_{i}, g_{i+1}\rangle -
    \tfrac{2\alpha_i - B}{2h_i} \|g_{i}-g_{i+1}\|^{2} 
    + 
    % \right. \\ & \left. \qquad  \qquad
    \Big[
    \tfrac{-(2\alpha_i - B)\kappa h_i}{2} + 
    (1+\kappa)\alpha_i - B
    +\tfrac{(1-\kappa)L}{h_i} \sigma_i\Big] \|g_i\|^2
    \right\} + \\
    %%%%
    %%%%
    &\left(1-\kappa\right)\left(\sigma_N - B \tfrac{1}{2L}\right)\|g_N\|^2 
        {{}\leq{}} 0
\end{aligned} %\label{eq:general_ineq_to_proove}
\end{align*}
}%
Further, we multiply the inequality by 2 and form the squares in every inner term of the sum:
{\small
\begin{align}
% \hspace{-0.7in}
\begin{aligned}\label{eq:identity_middle_proof_squares}
    & \tfrac{h_i}{L}
    \left\{
    -2\left[
    (1+\kappa)\alpha_i-\kappa B
    \right]  \langle g_{i}, g_{i+1}\rangle 
    -\tfrac{2\alpha_i - B}{h_i} \|g_{i}-g_{i+1}\|^{2}
    +
    % \right. \\ & \left. \qquad  
    \left[
    - (2\alpha_i - B) \kappa h_i + 
    2\left[(1+\kappa)\alpha_i-B\right] + 
    \tfrac{2\left(1-\kappa\right)L}{h_i}\sigma_i
    \right] \|g_i\|^2
    \right\} = \\
    & \left\{-\tfrac{2\alpha_i - B}{L} + \tfrac{h_i}{L}\left[(1+\kappa)\alpha_i-\kappa B\right]\right\}\ \|g_{i}-g_{i+1}\|^{2} + 
    \\ &
    \,\, \tfrac{h_i}{L} \left\{
    \left[
    - (2\alpha_i - B) \kappa h_i  + 
    2\left[(1+\kappa)\alpha_i-B\right] + 
    \tfrac{2\left(1-\kappa\right)L}{h_i}\sigma_i
    \right]
    - \left[
    (1+\kappa)\alpha_i-\kappa B
    \right]
    \right\} \|g_i\|^2 - \\
    & \,\,\tfrac{h_i}{L} \left[(1+\kappa)\alpha_i-\kappa B\right]\, \|g_{i+1}\|^2
\end{aligned}
\end{align}
}%
Then we replace the identity \eqref{eq:identity_middle_proof_squares} in the inequality and adjust the indices of the gradients:
{\normalsize
\begin{align*}
    \begin{aligned}
    & \sum\limits_{i=0}^{N-1} \left\{-\tfrac{2\alpha_i - B}{L} + \tfrac{h_i}{L}\left[(1+\kappa)\alpha_i-\kappa B\right]\right\} \|g_{i}-g_{i+1}\|^{2} + \\
    & 2\left(1-\kappa\right)\left(\sigma_N - B \tfrac{1}{2L}\right)\|g_N\|^2 + \\
    &\sum\limits_{i=0}^{N-1} \tfrac{h_i}{L} \left\{
    \left[
    - (2\alpha_i - B) \kappa h_i  + 
    2\left[(1+\kappa)\alpha_i-B\right] + 
    \tfrac{2\left(1-\kappa\right)L}{h_i}\sigma_i
    \right]
    - \left[
    (1+\kappa)\alpha_i-\kappa B
    \right]
    \right\} \|g_i\|^2 - \\
    & \sum\limits_{i=1}^{N} \tfrac{h_{i-1}}{L} \left[(1+\kappa)\alpha_{i-1}-\kappa B\right] \|g_{i}\|^2 {{}\leq{}} 0
    \end{aligned}
\end{align*}
}%
For simplicity, we divide the inequality by $\frac{B}{L} > 0$ and define the scalars $T_1$, $T_2$, $T_3$ and $T_4$ that multiply the squared gradient norms. Showing that these scalars are non-positive will finish the proof.
{\small
\begin{align}\label{eq:main_ineq_to_prove}
    \begin{aligned}
    & \sum\limits_{i=0}^{N-1} \underbrace{ \Big\{-\left(2\tfrac{\alpha_i}{B} - 1\right) + h_i\Big[(1+\kappa)\tfrac{\alpha_i}{B}-\kappa \Big]\Big\}}_{T_1:=} \|g_{i}-g_{i+1}\|^{2} + \\
    &\sum\limits_{i=1}^{N-1} 
   \underbrace{ \left(
    h_i
    \Big[
    - \left(2\tfrac{\alpha_i}{B} - 1\right) \kappa h_i  + 
    2\Big[(1+\kappa)\tfrac{\alpha_i}{B}-1\Big] + 
    \tfrac{2L\left(1-\kappa\right)}{h_i B}\sigma_i
    \Big]
    - h_i \Big[
    (1+\kappa)\tfrac{\alpha_i}{B}-\kappa
    \Big]
     - h_{i-1} \Big[(1+\kappa)\tfrac{\alpha_{i-1}}{B}-\kappa \Big]
    \right)
    }_{T_2:=}
    \|g_i\|^2 + \\
    & + \underbrace{\left(2\left(1-\kappa\right)\left(\tfrac{\sigma_N L}{B} - \tfrac{1}{2}\right) - h_{N-1} \Big[(1+\kappa)\tfrac{\alpha_{N-1}}{B}-\kappa \Big] \right)}_{T_3:=}
    \|g_{N}\|^2 + \\
    & + h_0 \underbrace{\Big\{
    \Big[
    - \left(2\tfrac{\alpha_0}{B} - 1\right) \kappa h_0  + 
    2\Big[(1+\kappa)\tfrac{\alpha_0}{B}-1\Big] + 
    \tfrac{2L\left(1-\kappa\right)}{h_0 B}\sigma_0
    \Big]
    - \Big[
    (1+\kappa)\tfrac{\alpha_0}{B}-\kappa
    \Big]
    \Big\}}_{T_4:=} \|g_0\|^2 {{}\leq{}} 0
    \end{aligned} 
\end{align}
}%
For every coefficient $T_i$ we study the two possible cases: $0 < h_i {}\leq{} 1$ and $1 {}\leq{} h_i {}\leq{} \bar{h}(\kappa)$, respectively.

\begin{enumerate}[wide, labelindent=0pt]
    \item $T_1 = -\left(2\tfrac{\alpha_i}{B} - 1\right) + h_i\left[(1+\kappa)\tfrac{\alpha_i}{B}-\kappa \right]$
    \begin{enumerate}
        \item For $h_i {}\leq{} 1$, $\tfrac{\alpha_i}{B} = 1$, hence:
        {\normalsize
        \begin{align*}
        \begin{aligned}
            T_1\left(h_i {}\leq{} 1\right) = -1 + h_i {}\leq{} 0
        \end{aligned}
        \end{align*}
        }
        \item For $h_i {}\geq{} 1$, $\tfrac{\alpha_i}{B} = \tfrac{1-\kappa h_i}{2-(1+\kappa)h_i}$ and
        {\normalsize
        \begin{align*}
        \hspace{-0.7in}
        \begin{aligned}
            T_1\left(h_i {}\geq{} 1\right) 
            =
            -\left[\tfrac{2-2\kappa h_i}{2-(1+\kappa)h_i}-1\right] + 
            h_i \left[
            (1+\kappa) \tfrac{1-\kappa h_i}{2-(1+\kappa)h_i} - \kappa 
            \right] 
            %\\
            % &= -\left[\tfrac{2-2\kappa h_i -2 + (1+\kappa)h_i}{2-(1+\kappa)h_i}\right] + 
            % h_i \left[
            % \tfrac{1-\kappa h_i + \kappa - \kappa^2 h_i - 2\kappa + \kappa(1+\kappa)h_i}
            % {2-(1+\kappa)h_i}
            % \right] \\
            % &= -\tfrac{(1-\kappa)h_i}{2-(1+\kappa)h_i} + 
            % h_i 
            % \tfrac{1 - \kappa}
            % {2-(1+\kappa)h_i}
             = 0.
        \end{aligned}
        \end{align*}
        }
    \end{enumerate}
    Hence $T_1 {}\leq{} 0$, $\forall h_i \in \big(0, \bar{h}(\kappa)\big]$.
    
    % \clearpage
    \item {\normalsize{$T_2 = 
    \underbrace{
    h_i
    \big[
    - \big(2\tfrac{\alpha_i}{B} - 1\big) \kappa h_i  + 
    2\big[(1+\kappa)\tfrac{\alpha_i}{B}-1\big] + 
    \tfrac{2L\left(1-\kappa\right)}{h_i B}\sigma_i
    \big]
    }_{D:=}
    - h_i \big[
    (1+\kappa)\tfrac{\alpha_i}{B}-\kappa
    \big]
     - h_{i-1} \big[(1+\kappa)\tfrac{\alpha_{i-1}}{B}-\kappa \big]$}}
    
    In the analysis of $T_2$, there are four possible cases due to the two choices of $h_i$ and $h_{i+1}$, i.e., $h_{i,i+1} \lessgtr 1$. The identity $\eqref{eq:identity_norm_gi_multipliers_over_B}$ is derived by just replacing the expressions of $\alpha_i$ and $B$ for every possible case.
    {\normalsize
    \begin{align}\label{eq:identity_norm_gi_multipliers_over_B}
    D
    = 
    \max
    \left\{
    h_i+h_{i-1},\, 
    \tfrac{2(1-\kappa)\left(h_i+h_{i-1} - (1+\kappa)h_i h_{i-1}\right)}
    {(2-(1+\kappa)h_{i-1})\ (2-(1+\kappa)h_i)}
    \right\}
\end{align}
}%
    \begin{enumerate}
        \item For $h_i {}\leq{} 1$, $\tfrac{\alpha_i}{B}=1$ and from \eqref{eq:identity_norm_gi_multipliers_over_B} we get $D=h_i+h_{i-1}$.
        {\normalsize
        \begin{align*}
            \begin{aligned}
            T_2(h_i {}\leq{} 1) 
            {}={} h_i+h_{i-1}
            -{h_i}
            -{h_{i-1}} \left[
            (1+\kappa)\tfrac{\alpha_{i-1}}{B}-\kappa 
            \right] 
            % \\ &
            {}={} h_{i-1} (1+\kappa) \left(1-\tfrac{\alpha_{i-1}}{B}\right)
            \end{aligned}
        \end{align*}
        }
        We next proceed to the two subcases:
        \begin{enumerate}
            \item If $h_{i-1} {}\leq{} 1$, then $\tfrac{\alpha_{i-1}}{B}=1$ and 
            $$
            T_2(h_i {}\leq{} 1, h_{i-1} {}\leq{} 1)=0
            $$
            \item If $h_{i-1} {}\geq{} 1$, then $\tfrac{\alpha_{i-1}}{B} = \tfrac{1-\kappa h_{i-1}}{2-(1+\kappa)h_{i-1}}$. Then
            {\normalsize
            \begin{align*}
                T_2(h_i {}\leq{} 1, h_{i-1} {}\geq{} 1) = h_{i-1} (1+\kappa) \tfrac{1-h_{i-1}}{2-(1+\kappa)h_{i-1}} {}\leq{} 0
            \end{align*}
            }
        \end{enumerate}
        
        \item For $h_i {}\geq{} 1$, $\tfrac{\alpha_{i}}{B} = \tfrac{1-\kappa h_i}{2-(1+\kappa)h_i}$ and from \eqref{eq:identity_norm_gi_multipliers_over_B} we get 
        $D= \tfrac{2(1-\kappa)\left(h_i+h_{i-1} - (1+\kappa)h_i h_{i-1}\right)}
    {(2-(1+\kappa)h_{i-1})\ (2-(1+\kappa)h_i)}$. After direct algebraic manipulations, one obtains
    {\normalsize
        \begin{align*}
            \hspace{-1cm}
            \begin{aligned}
            T_2(h_i {}\geq{} 1) 
    %         &= \tfrac{2(1-\kappa)\left(h_i+h_{i-1} - (1+\kappa)h_i h_{i-1}\right)}
    % {(2-(1+\kappa)h_{i-1})\ (2-(1+\kappa)h_i)}
    %         -h_i \left[
    %         (1+\kappa)\tfrac{1-\kappa h_i}{2-(1+\kappa)h_i}-\kappa
    %         \right]
    %         -h_{i-1} \left[
    %         (1+\kappa)\tfrac{\alpha_{i-1}}{B}-\kappa 
    %         \right]\\
    %             &= \tfrac{2(1-\kappa)\left({h_i}+{h_{i-1}}-(1+\kappa){h_i}{h_{i-1}}\right)}
    % {(2-(1+\kappa){h_{i-1}})\ (2-(1+\kappa)h_i)}
    %         -{h_i} \left[
    %         \tfrac{1-\kappa }{2-(1+\kappa)h_i}
    %         \right]
    %         -{h_{i-1}} \left[
    %         (1+\kappa)\tfrac{\alpha_{i-1}}{B}-\kappa 
    %         \right] \\
    %             &= \tfrac{1-\kappa }{2-(1+\kappa)h_i}
    %             \left[
    %             \tfrac{2\left({h_i}+{h_{i-1}}-(1+\kappa){h_i}{h_{i-1}}\right)}
    % {2-(1+\kappa){h_{i-1}}} - {h_i}
    %             \right] 
    %             -{h_{i-1}} \left[
    %         (1+\kappa)\tfrac{\alpha_{i-1}}{B}-\kappa 
    %         \right] \\
    %             &= \tfrac{1-\kappa }{2-(1+\kappa)h_i}\  
    %             \tfrac{2{h_{i-1}}-(1+\kappa)h_{i}h_{i-1}}{2-(1+\kappa){h_{i-1}}}
    %             - {h_{i-1}} \left[
    %         (1+\kappa)\tfrac{\alpha_{i-1}}{B}-\kappa 
    %         \right] \\ &
                = {h_{i-1}}
                \left[
                \tfrac{1-\kappa }{2-(1+\kappa)h_{i-1}}
                    - \big(
                (1+\kappa)\tfrac{\alpha_{i-1}}{B}-\kappa 
                \big)
                \right] 
            \end{aligned}
        \end{align*}
        }%
        We next proceed to the two subcases:
        \begin{enumerate}
            \item If $h_{i-1} {}\leq{} 1$, then $\tfrac{\alpha_{i-1}}{B}=1$, hence
            {\normalsize
            \begin{align*}
                T_2(h_i {}\geq{} 1, h_{i-1} {}\leq{} 1) 
                % &= {h_{i-1}}
                % \left[
                % \tfrac{1-\kappa }{2-(1+\kappa)h_{i-1}}
                %     - 1
                % \right] 
                = (1+\kappa){h_{i-1}} \tfrac{-1+h_{i-1}}{2-(1+\kappa){h_{i-1}}} {}\leq{} 0
            \end{align*}
            }
            
            \item If $h_{i-1} {}\geq{} 1$, then $\tfrac{\alpha_{i-1}}{B} = \tfrac{1-\kappa h_{i-1}}{2-(1+\kappa)h_{i-1}}$. 
            and by direct computations we obtain
            {\normalsize
            \begin{align*}
                T_2(h_i {}\geq{} 1, h_{i-1} {}\geq{} 1) 
                % &= {h_{i-1}}
                % \left[
                % \tfrac{1-\kappa }{2-(1+\kappa)h_{i-1}}
                %     - \left(
                % (1+\kappa)\tfrac{1-\kappa h_{i-1}}{2-(1+\kappa)h_{i-1}}-\kappa 
                % \right)
                % \right] 
                % \\
                % &= {h_{i-1}}
                % \left[
                % \tfrac{1-\kappa }{2-(1+\kappa)h_{i-1}}
                %     - \tfrac{1-\kappa}{2-(1+\kappa)h_{i-1}}
                % \right] 
                = 0
            \end{align*}
            }
            
        \end{enumerate}
        
    \end{enumerate}
    Hence, $T_2 {}\leq{} 0$, $\forall h_i \in \big(0, \bar{h}(\kappa)\big]$.
    %%%%%%%%%%%
    % \clearpage
    \item $T_3 =2\left(1-\kappa\right)\left(\tfrac{\sigma_N L}{B} - \tfrac{1}{2}\right) - h_{N-1} \left[(1+\kappa)\tfrac{\alpha_{N-1}}{B}-\kappa \right]$
    \begin{enumerate}
        \item ${h_{N-1}} {}\leq{} 1$: The following expressions for $\sigma_N$ and $\alpha_{N-1}$ state:
        {\normalsize
        \begin{align*}
            \begin{aligned}
            \tfrac{2L\sigma_N}{B} = 1 + \tfrac{h_{N-1}}{1-\kappa}\,\,,
            \qquad
            \tfrac{\alpha_{N-1}}{B} = 1
            \end{aligned}
        \end{align*}
        }
        By replacing them in the expression of $T_3$, we obtain
        {\normalsize
        \begin{align*}
            \begin{aligned}
            T_3(h_{N-1} {}\leq{} 1) 
            % = {h_{N-1}} - {h_{N-1}} \left[(1+\kappa)-\kappa \right] 
            = 0
            \end{aligned}
        \end{align*}
        }
        
        \item ${h_{N-1}} {}\geq{} 1$: The following expressions for $\sigma_N$ and $\alpha_{N-1}$ state:
        {\normalsize
        \begin{align*}
            \begin{aligned}
            \tfrac{2L\sigma_N}{B} = 1 + h_{N-1} \tfrac{1}{2-(1+\kappa)h_{N-1}}\,\,, \qquad
            \tfrac{\alpha_{N-1}}{B} = \tfrac{1-\kappa h_{N-1}}{2-(1+\kappa) h_{N-1}}
            \end{aligned}
        \end{align*}
        }
        By replacing them in the expression of $T_3$ we get
        {\normalsize
        \begin{align*}
            \begin{aligned}
            T_3(h_{N-1} {}\geq{} 1) 
            % &= h_{N-1}\Big[ 
            % \tfrac{1-\kappa}{2-(1+\kappa)h_{N-1}} -
            % \tfrac{(1+\kappa)(1-\kappa h_{N-1})}{2-(1+\kappa){h_{N-1}}} + \kappa
            % \Big] 
            % \\
            % &= {h_{N-1}} \left[ 
            % \tfrac{1-\kappa}{2-(1+\kappa){h_{N-1}}} -
            % \tfrac{\left(1-\kappa\right)}{2-(1+\kappa) {h_{N-1}}}
            % \right] 
            = 0
            \end{aligned}
        \end{align*}
        }
    \end{enumerate}
    Hence, $T_3=0$, $\forall h_i \in \big(0, \bar{h}(\kappa)\big]$.
    
    %%%%%%%%%%%%
    % \clearpage
    \item $T_4 = \big[
    - \big(2\tfrac{\alpha_0}{B} - 1\big) \kappa h_0  + 
    2\big[(1+\kappa)\tfrac{\alpha_0}{B}-1\big] + 
    \tfrac{2L(1-\kappa)}{h_0 B}\sigma_0
    \big]
    - \big[
    (1+\kappa)\tfrac{\alpha_0}{B}-\kappa
    \big]$
    \begin{enumerate}
        \item For $h_i {}\leq{} 1$, the following expressions for $\sigma_0$ and $\alpha_{0}$ state:
        {\normalsize
        \begin{align*}
            \begin{aligned}
                \tfrac{\sigma_0 L}{h_0 B} = 1 - \tfrac{1 - \kappa h_0}{2\left(1-\kappa\right)}
                \,\,,\qquad
                \tfrac{\alpha_0}{B} = 1
            \end{aligned}
        \end{align*}
        }
        We replace them in the expression of $T_4$ and obtain
        {\normalsize
        \begin{align*}
            \begin{aligned}
            T_4(h_i {}\leq{} 1) 
            % &=  \left[
            %     - \kappa h_0  + 
            %     2\kappa + 
            %     2\left(1-\kappa\right) - 1 + \kappa h_0
            %     \right]
            %     - 1 
                = 0
            \end{aligned}
        \end{align*}
        }
        
        \item For $h_i {}\geq{} 1$, the following expressions for $\sigma_0$ and $\alpha_{0}$ state:
        {\normalsize
        \begin{align*}
            \begin{aligned}
                \tfrac{\sigma_0 L}{h_0 B} 
                = 1 - \tfrac{1-\kappa h_0^2}{2\left[2-(1+\kappa)h_0\right]} 
                = \tfrac{\kappa h_0^2 - 2(1+\kappa)h_0 +  3}{2\left[2-(1+\kappa)h_0\right]}
                \,\,,\qquad
                \tfrac{\alpha_0}{B} = \tfrac{1-\kappa h_0}{2-(1+\kappa)h_0}
            \end{aligned}
        \end{align*}
        }
        We replace them in the expression of $T_4$ and after direct computations obtain:
        {\small
        \begin{align*}
            \begin{aligned}
            \hspace{-1cm}
            T_4(h_i {}\geq{} 1) 
            % &=  \left[
            %         - \left(2\tfrac{1-\kappa h_0}{2-(1+\kappa)h_0} - 1\right) \kappa h_0  + 
            %         2\left[(1+\kappa)\tfrac{1-\kappa h_0}{2-(1+\kappa)h_0}-1\right] + 
            %         2\left(1-\kappa\right)\tfrac{\kappa h_0^2 - 2(1+\kappa)h_0 +  3}{2\left(2-(1+\kappa)h_0\right)}
            %         \right]
            %         - \left[
            %         (1+\kappa)\tfrac{1-\kappa h_0}{2-(1+\kappa)h_0}-\kappa
            %         \right] 
                    % \\
                % &=  \tfrac{-\kappa(1-\kappa)h_0^2}{2-(1+\kappa)h_0}  + 
                %     2\tfrac{-1 + \kappa -\kappa^2 h_0 + h_0}{2-(1+\kappa)h_0} + 
                %     \left(1-\kappa\right)\tfrac{\kappa h_0^2 - 2(1+\kappa)h_0 +  3}{2-(1+\kappa)h_0}
                %     - \tfrac{1-\kappa}{2-(1+\kappa)h_0} \\
                % &=  \tfrac{1-\kappa}{2-(1+\kappa)h_0} 
                % \left[
                %  {-\kappa h_0^2} \ + \ 
                %     2\left(-1 + (1+\kappa) h_0 \right) \ + \ 
                %     \kappa h_0^2 \ - \  2(1+\kappa)h_0 +  3 \ 
                %     - \ 1
                %     \right] \\
                = 0
            \end{aligned}
        \end{align*}
        }%
    \end{enumerate}
    Hence, $T_4=0$, $\forall h_i \in (0, \bar{h}(\kappa)]$.
\end{enumerate}%

To conclude, all terms from \eqref{eq:main_ineq_to_prove} are non-positive: 
\begin{itemize}
    \item $
    T_1 \left \{ 
    \arraycolsep=5pt
    
    \begin{array}{ll}
        = 0    & 1 {}\leq{} h_i {}\leq{} \frac{1+\kappa-\sqrt{1-\kappa+\kappa^2}}{\kappa} \\
        \leq 0 & h_i {}\leq{} 1
    \end{array}
    \right.
    $
    \item $
    T_2 \left \{ 
    \arraycolsep=5pt
    
    \begin{array}{ll}
        = 0    & (1-h_i)(1-h_{i-1}) {}\geq{} 0 \\
        \leq 0 & \text{ otherwise }
    \end{array}
    \right.
    $
    \item $T_3 = 0$
    \item $T_4 = 0$. 
\end{itemize}
Therefore, \eqref{eq:main_ineq_to_prove} is proved through a series of equivalent inequalities, hence $l {}\leq{} U$.

\end{proof}
